# Supplementary material for: Retrieval-Oriented Knowledge for Click-Through Rate Prediction
Source: arXiv:2404.18304 source file (2024-10-03)
Supplement: Supplementary file 1 [file 6Appendix.tex]

% \newpage
\section{Appendix}

\subsection{T-sne visualization}
Figure~\ref{fig:tsne_tmall} depict the knowledge distribution patterns of both \name and RIM in Tmall dataset. 
\begin{figure*}
\vspace{-10pt}
    \centering
    % Row 1
    % \begin{minipage}{0.5\textwidth}
    %     \begin{subfigure}{\linewidth}
    %         \includegraphics[width=0.49\linewidth]{figures/03Experiments/tsne/alipay/train/rim_tsne_plot_noncontra.pdf}
    %         \includegraphics[width=0.49\linewidth]{figures/03Experiments/tsne/alipay/train/rok_tsne_plot_noncontra.pdf}
    %     \end{subfigure}
    %     \subcaption{Alipay (Train)}
    % \end{minipage}%
    % \begin{minipage}{0.5\textwidth}
    %     \begin{subfigure}{\linewidth}
    %         \includegraphics[width=0.49\linewidth]{figures/03Experiments/tsne/alipay/test/rim_tsne_plot_noncontra.pdf}
    %         \includegraphics[width=0.49\linewidth]{figures/03Experiments/tsne/alipay/test/rok_tsne_plot_noncontra.pdf}
    %     \end{subfigure}
    %     \subcaption{Alipay (Test)}
    % \end{minipage}
    
    % Row 2 (if needed)
    \begin{minipage}{0.5\textwidth}
        \begin{subfigure}{\linewidth}
            \includegraphics[width=0.49\linewidth]{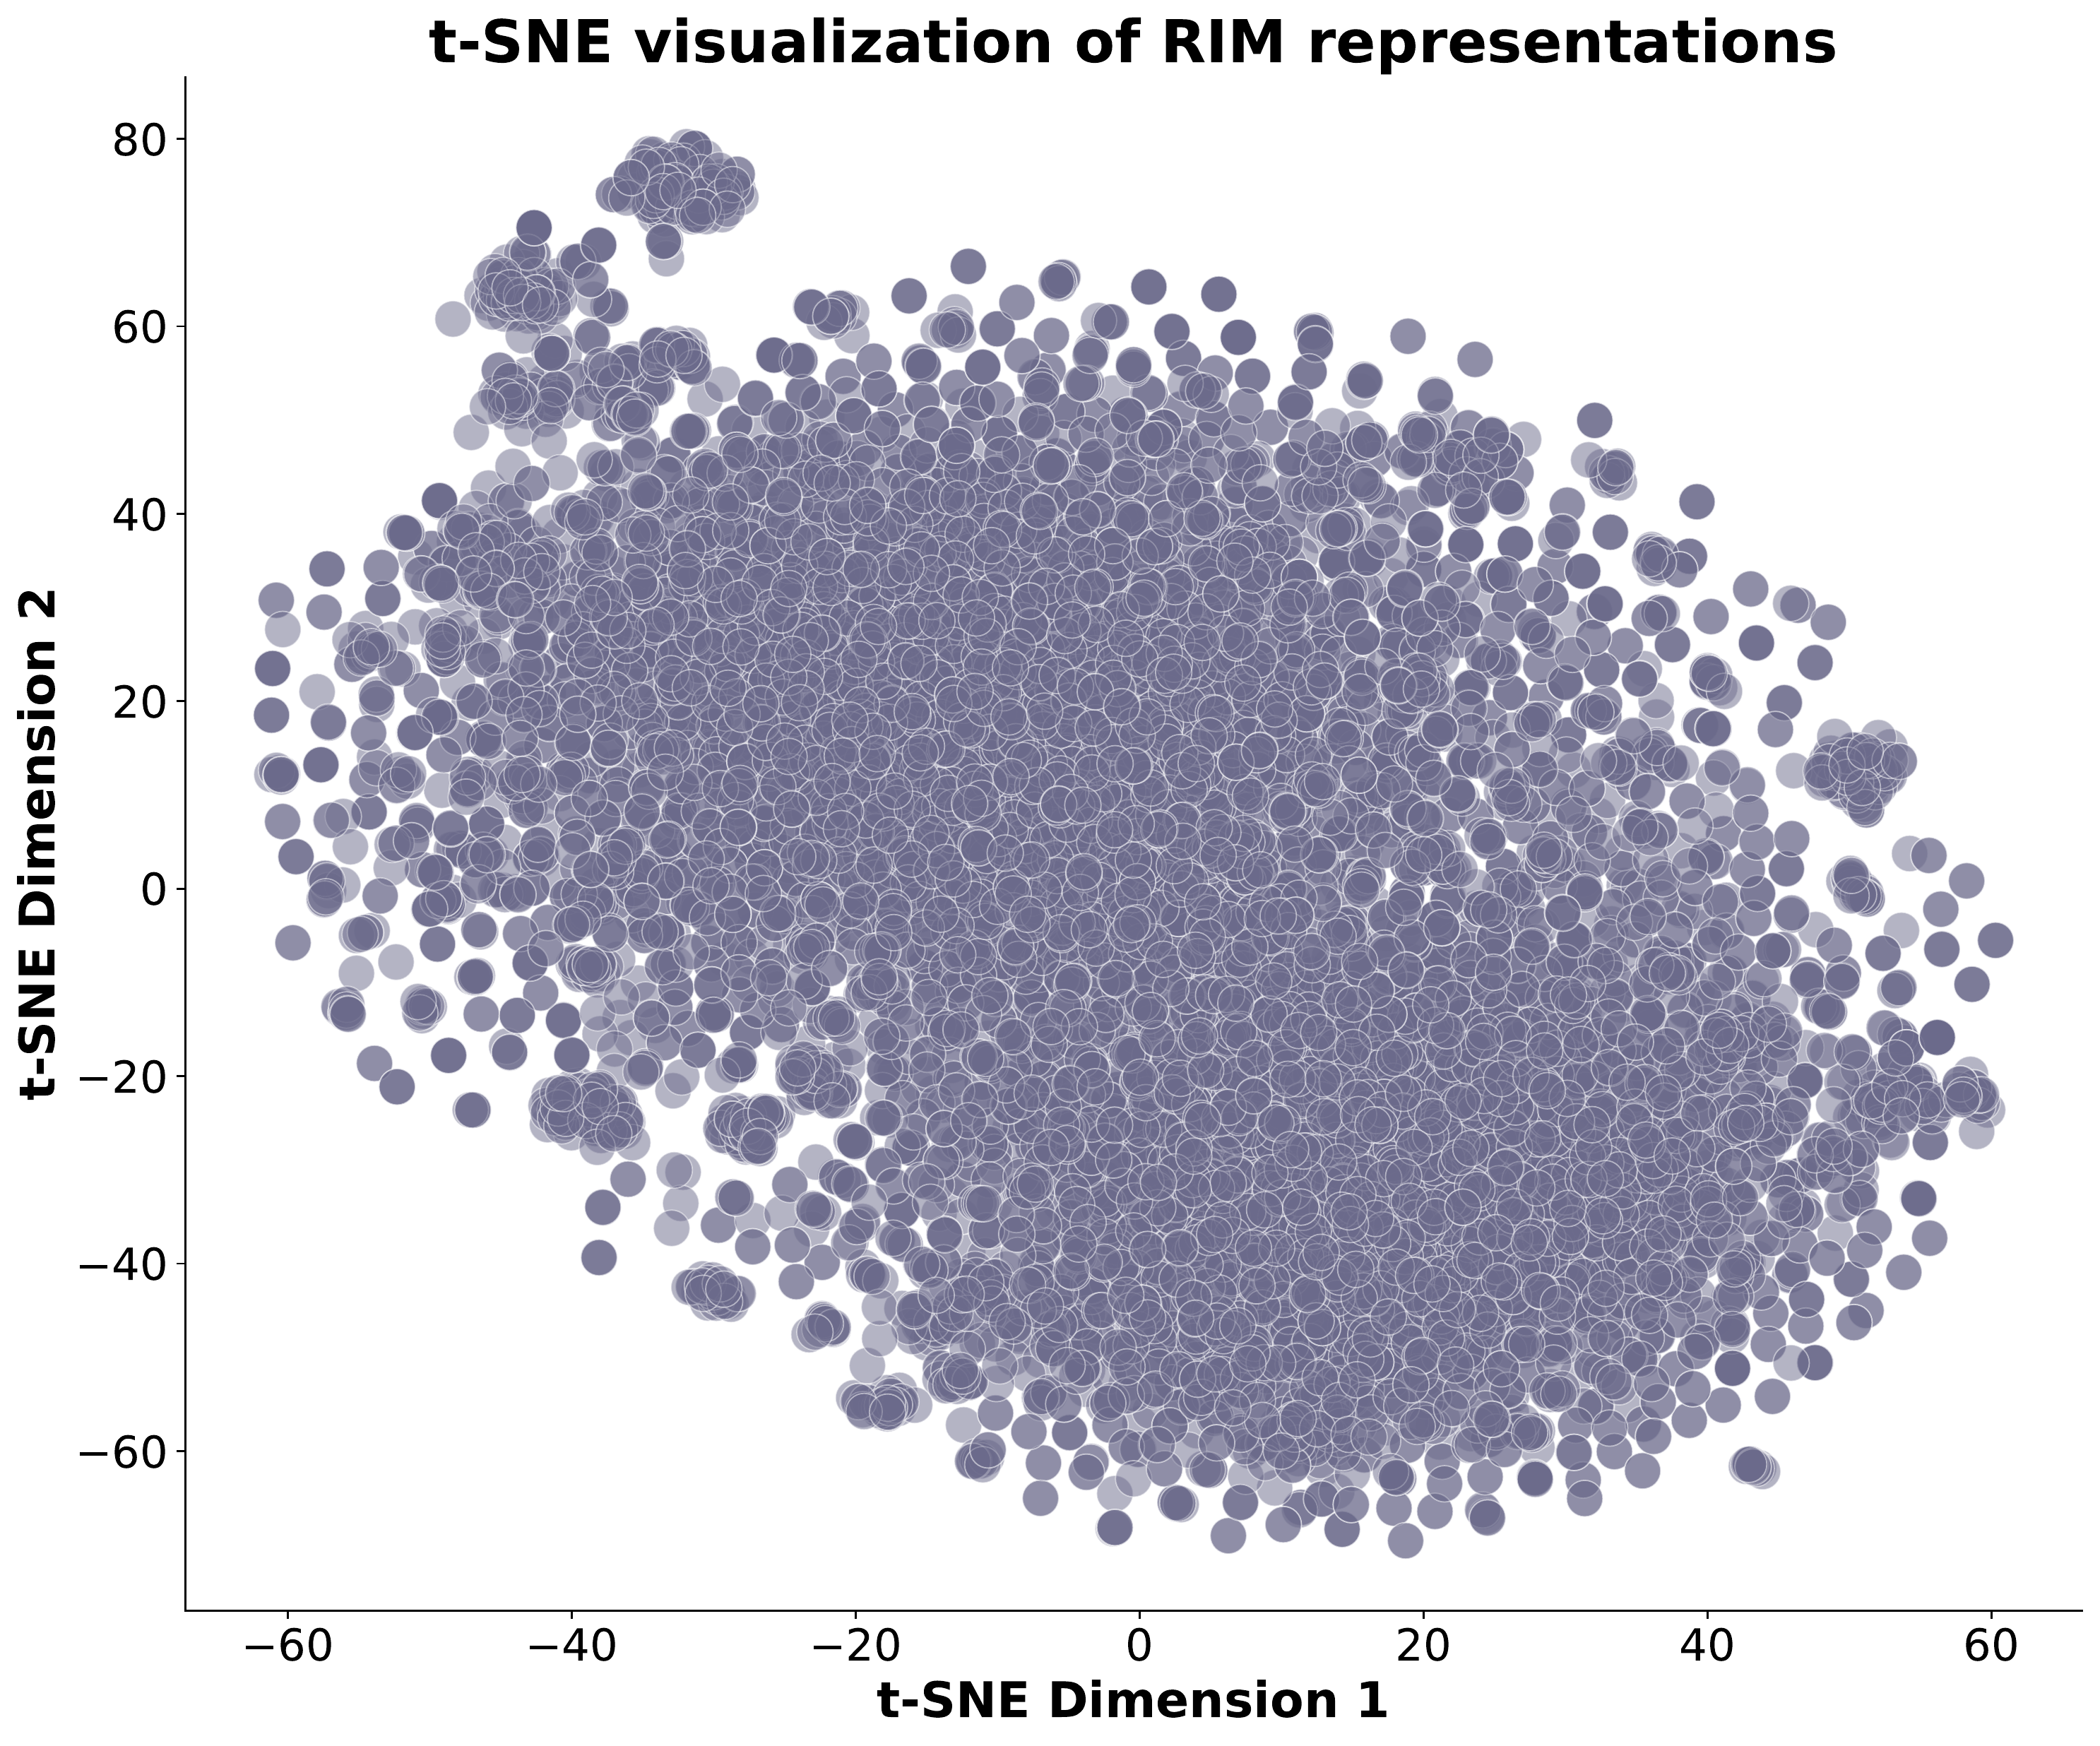}
            \includegraphics[width=0.49\linewidth]{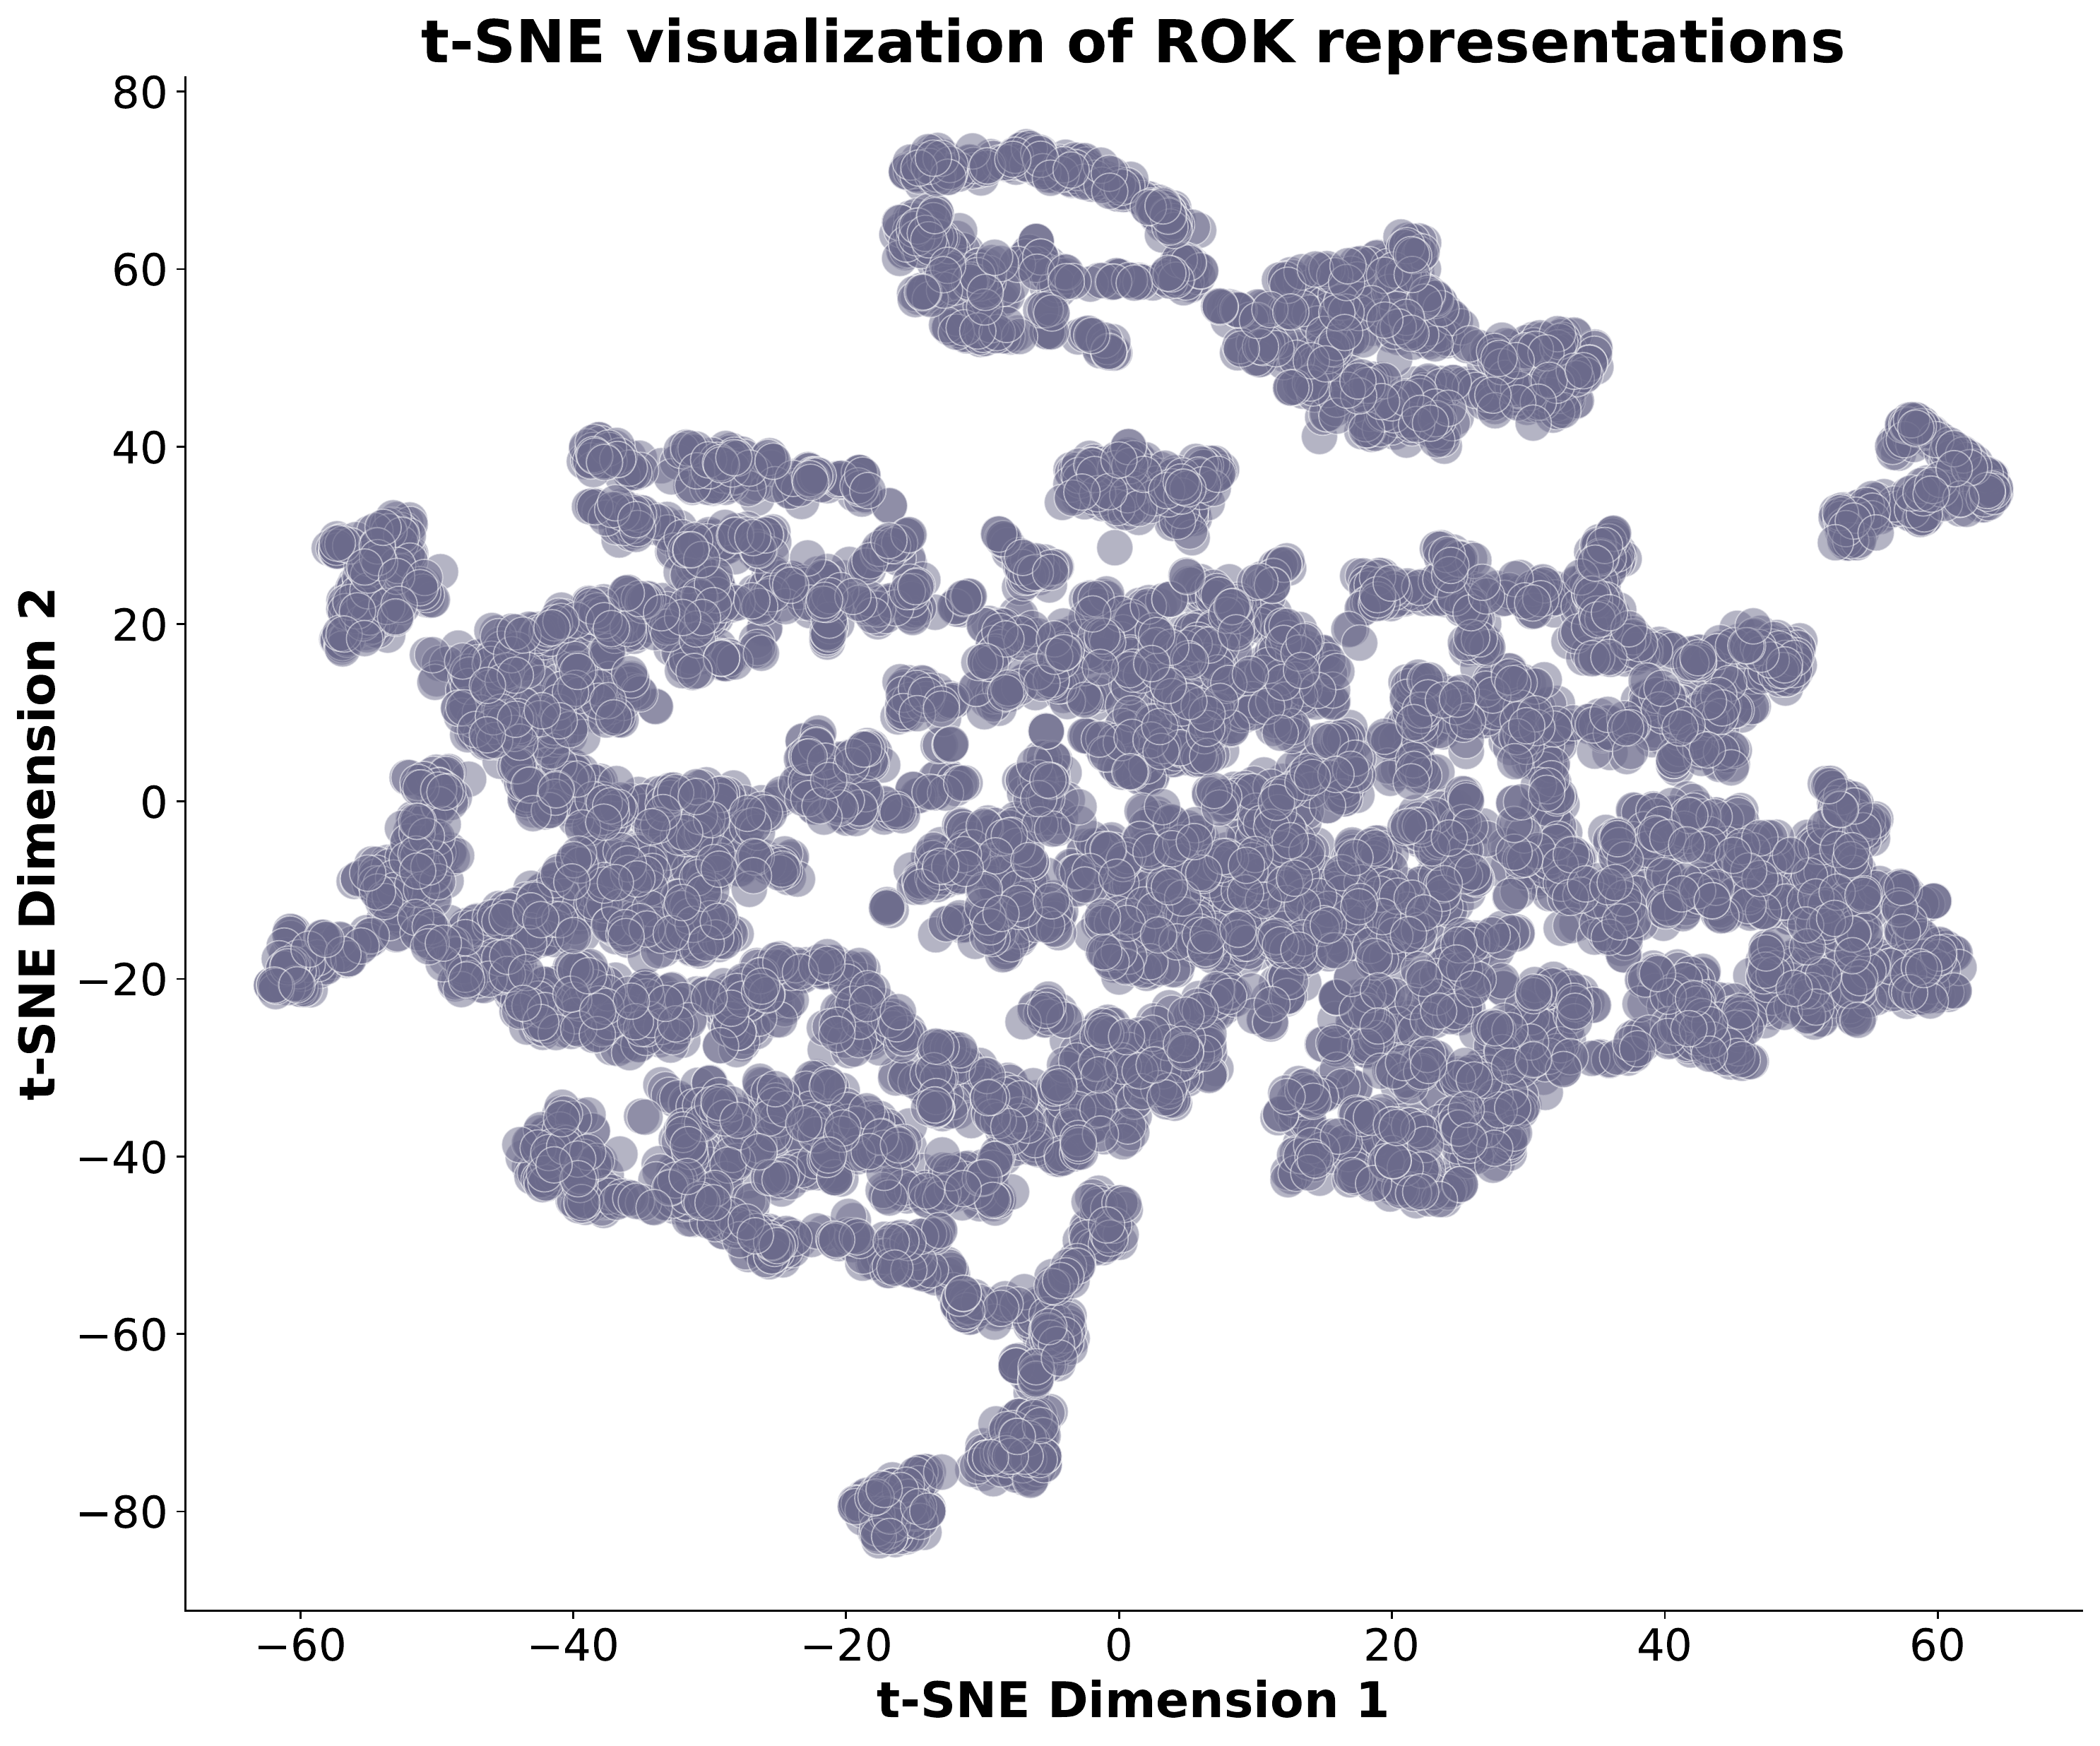}
        \end{subfigure}
        \subcaption{Tmall (Train)}
    \end{minipage}%
    \begin{minipage}{0.5\textwidth}
        \begin{subfigure}{\linewidth}
            \includegraphics[width=0.49\linewidth]{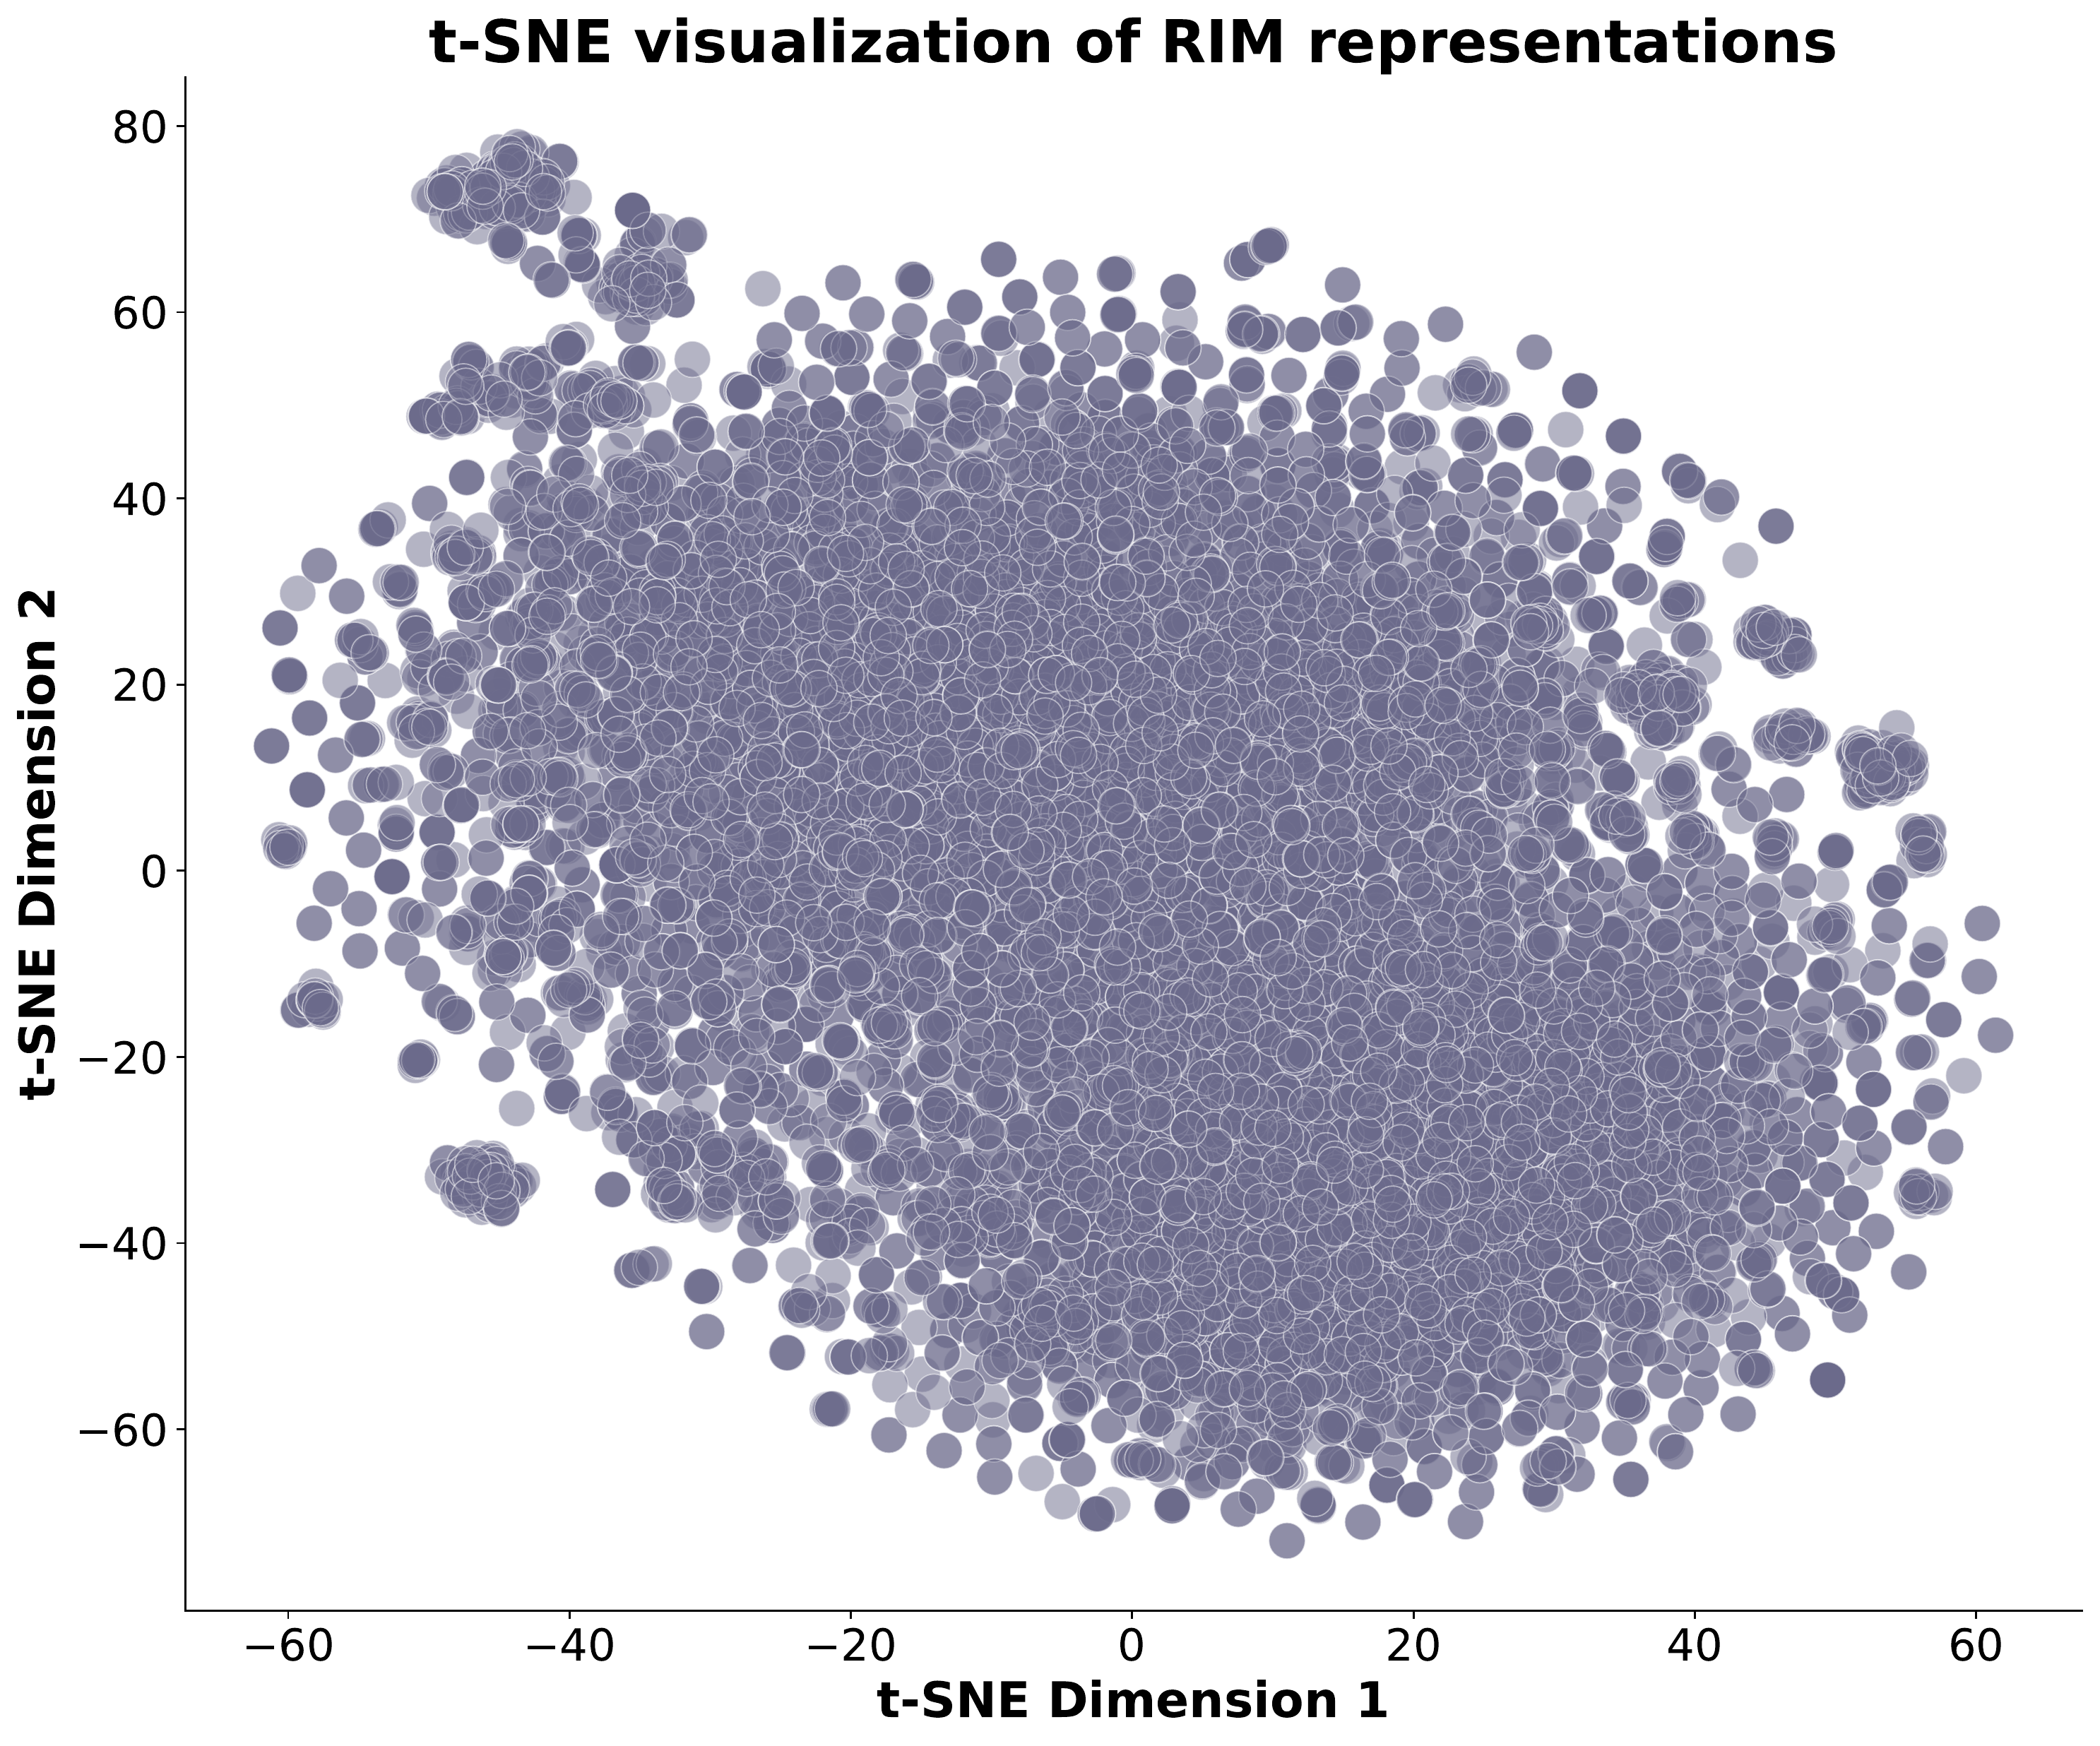}
            \includegraphics[width=0.49\linewidth]{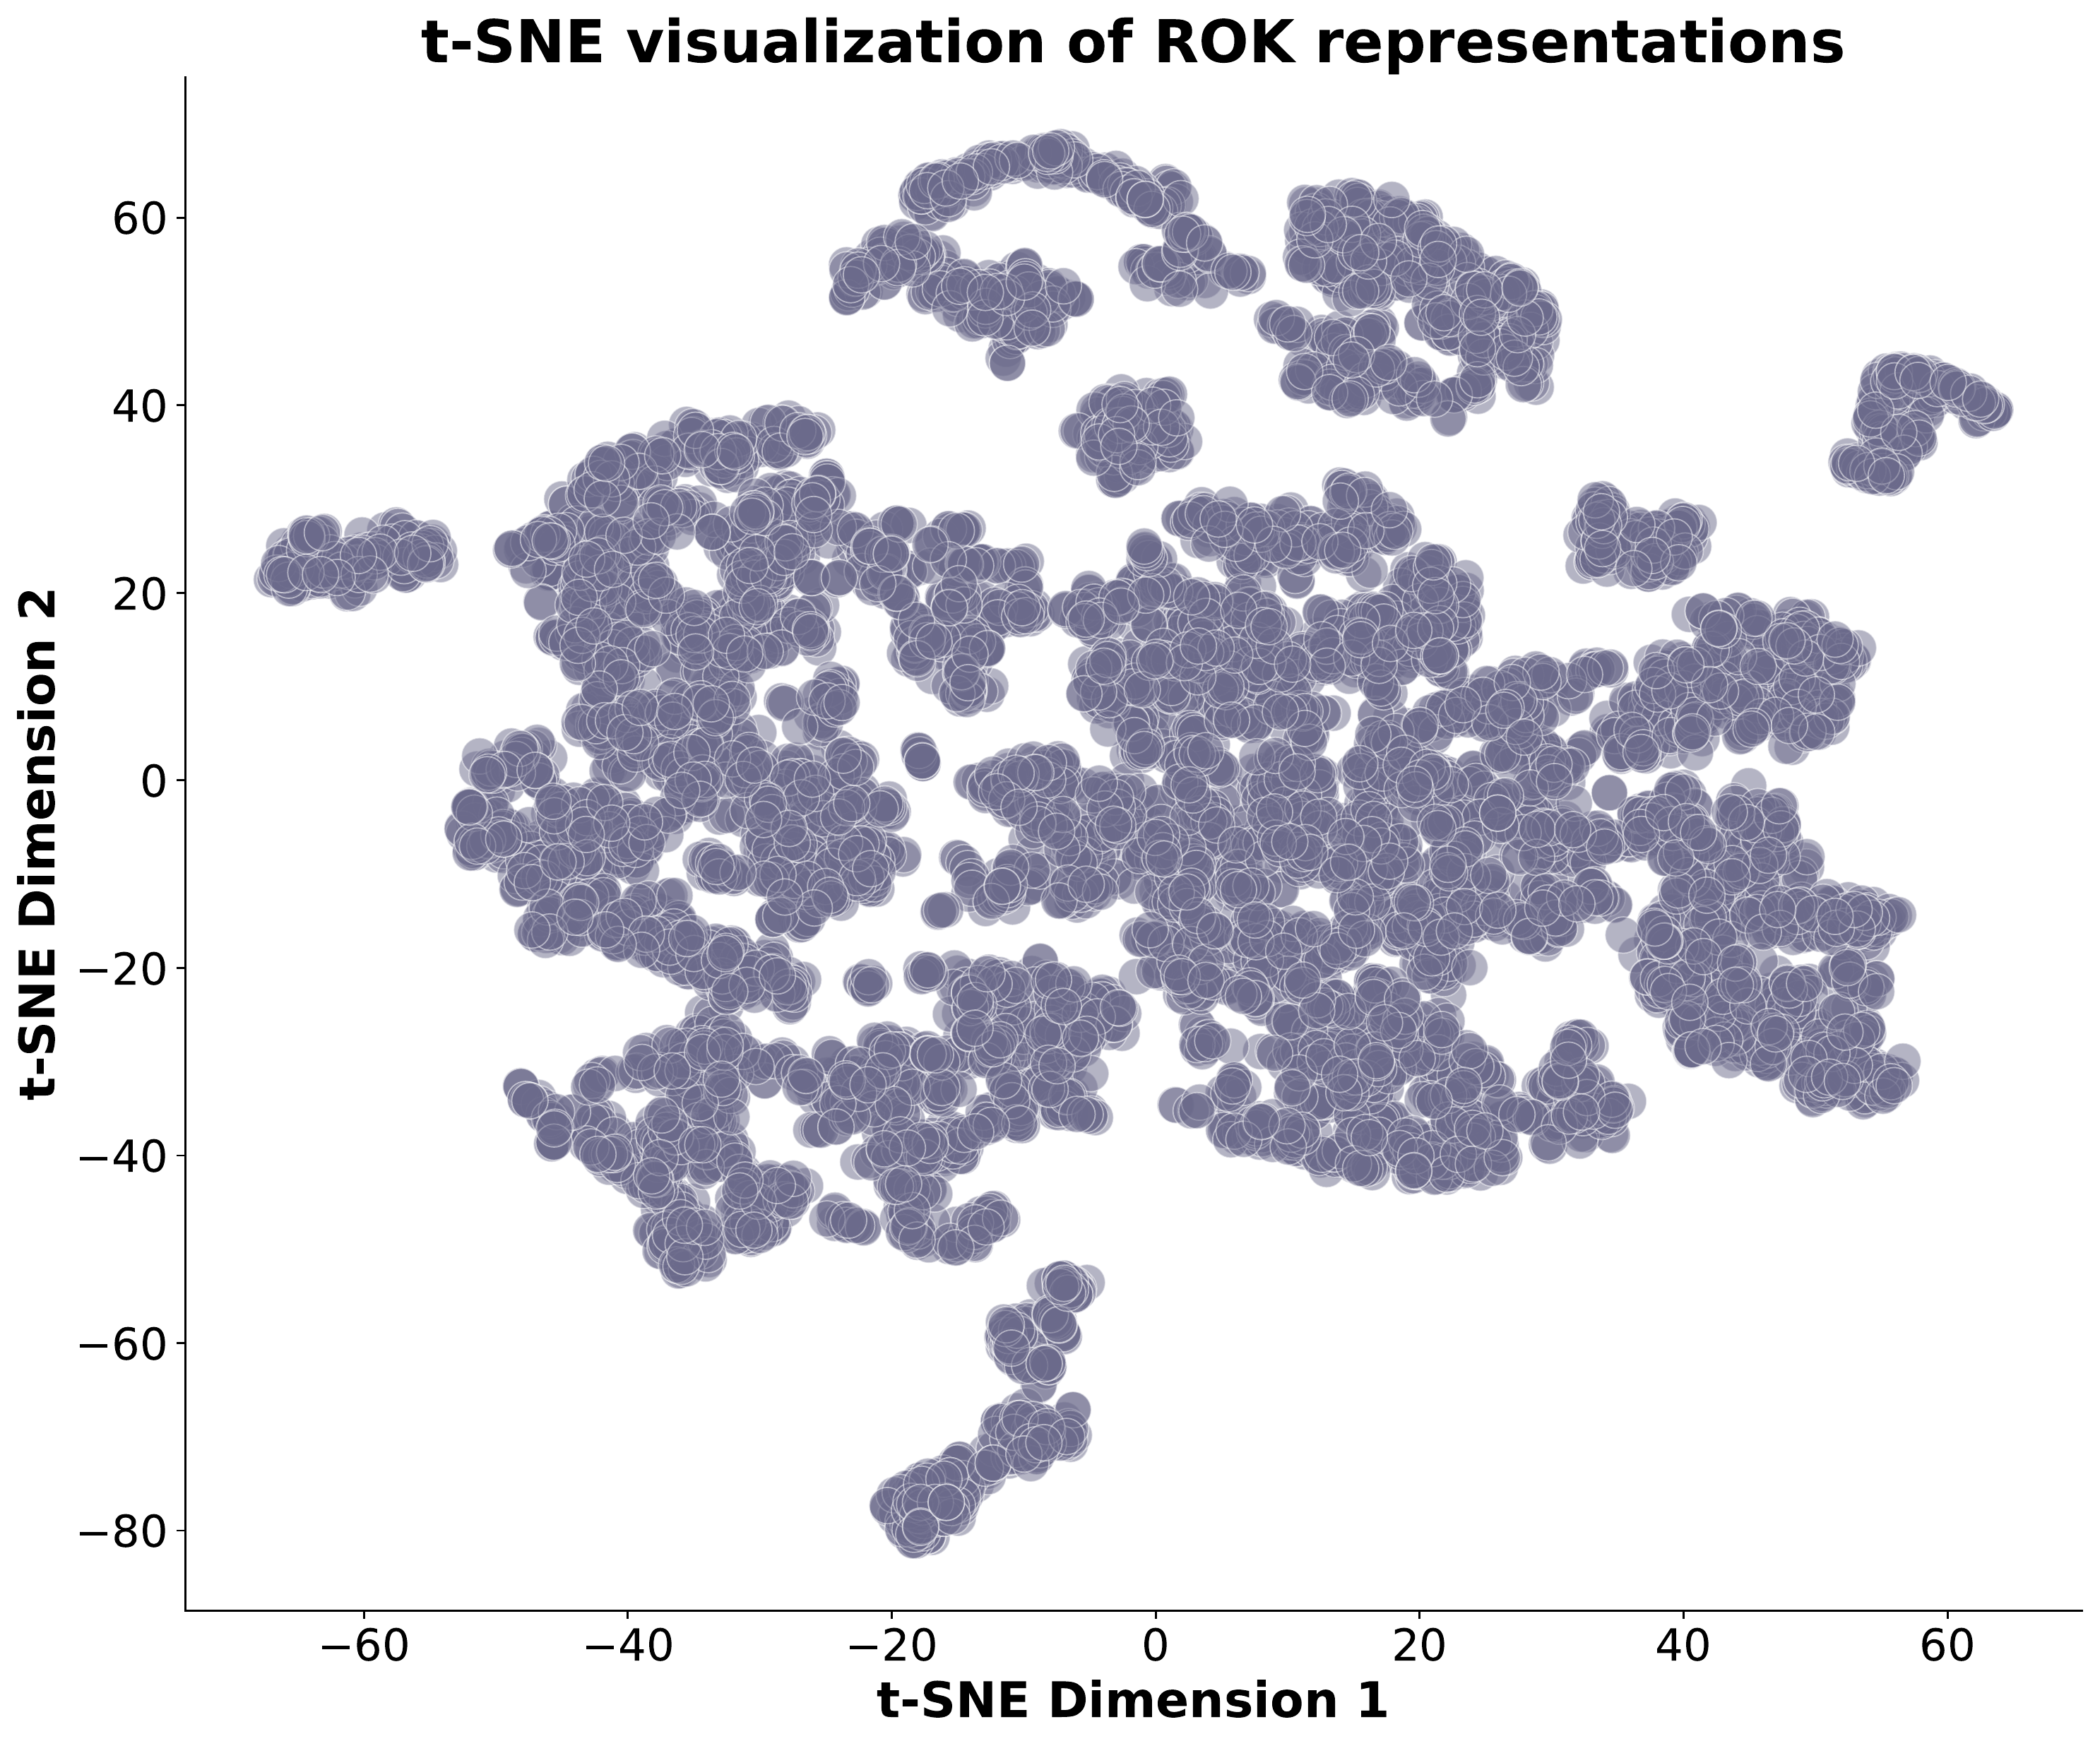}
        \end{subfigure}
        \subcaption{Tmall (Test)}
    \end{minipage}
    \caption{The t-SNE visualization of knowledge from RIM (on the left in each subfigure) and \name (on the right in each subfigure) for Tmall.}
    \label{fig:tsne_tmall}
    \vspace{-10pt}
\end{figure*}

\subsection{Ablation \& Hyper-parameter Study on Taobao}

In this section, we present the ablation and hyper-parameter study conducted on the Taobao dataset. The results are depicted in Figure~\ref{fig:update_strategy}, Figure~\ref{fig:alpha_values}.

% It's good practice to use descriptive labels for figures

\begin{figure}[H] % "htbp!" helps LaTeX to find the best possible location for the figure
    \centering
    \includegraphics[width=0.7\linewidth, height=\textheight, keepaspectratio]{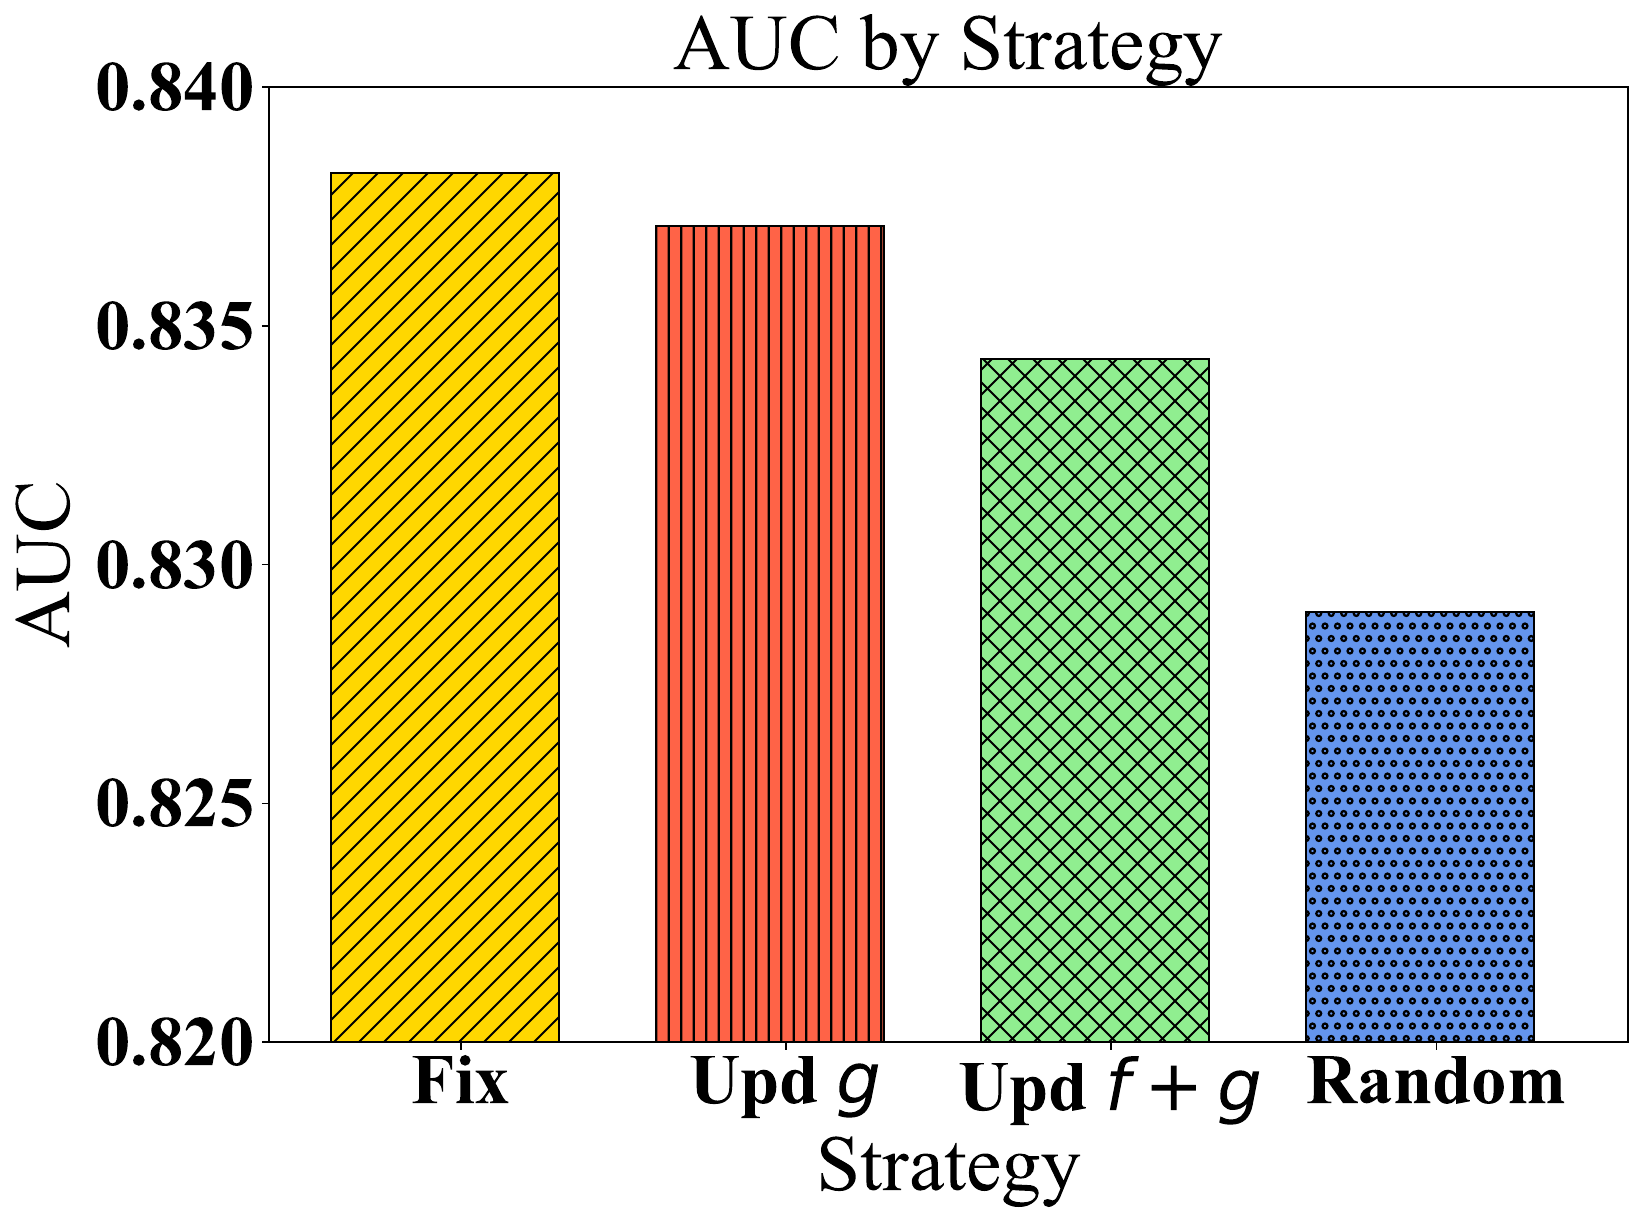} % Use textwidth to span the figure across the text width
    \caption{Comparison of AUC scores for different update strategies on Taobao.}
    \label{fig:update_strategy}
\end{figure}

\begin{figure}[H]
    \centering
    \includegraphics[width=0.7\linewidth, height=\textheight, keepaspectratio]{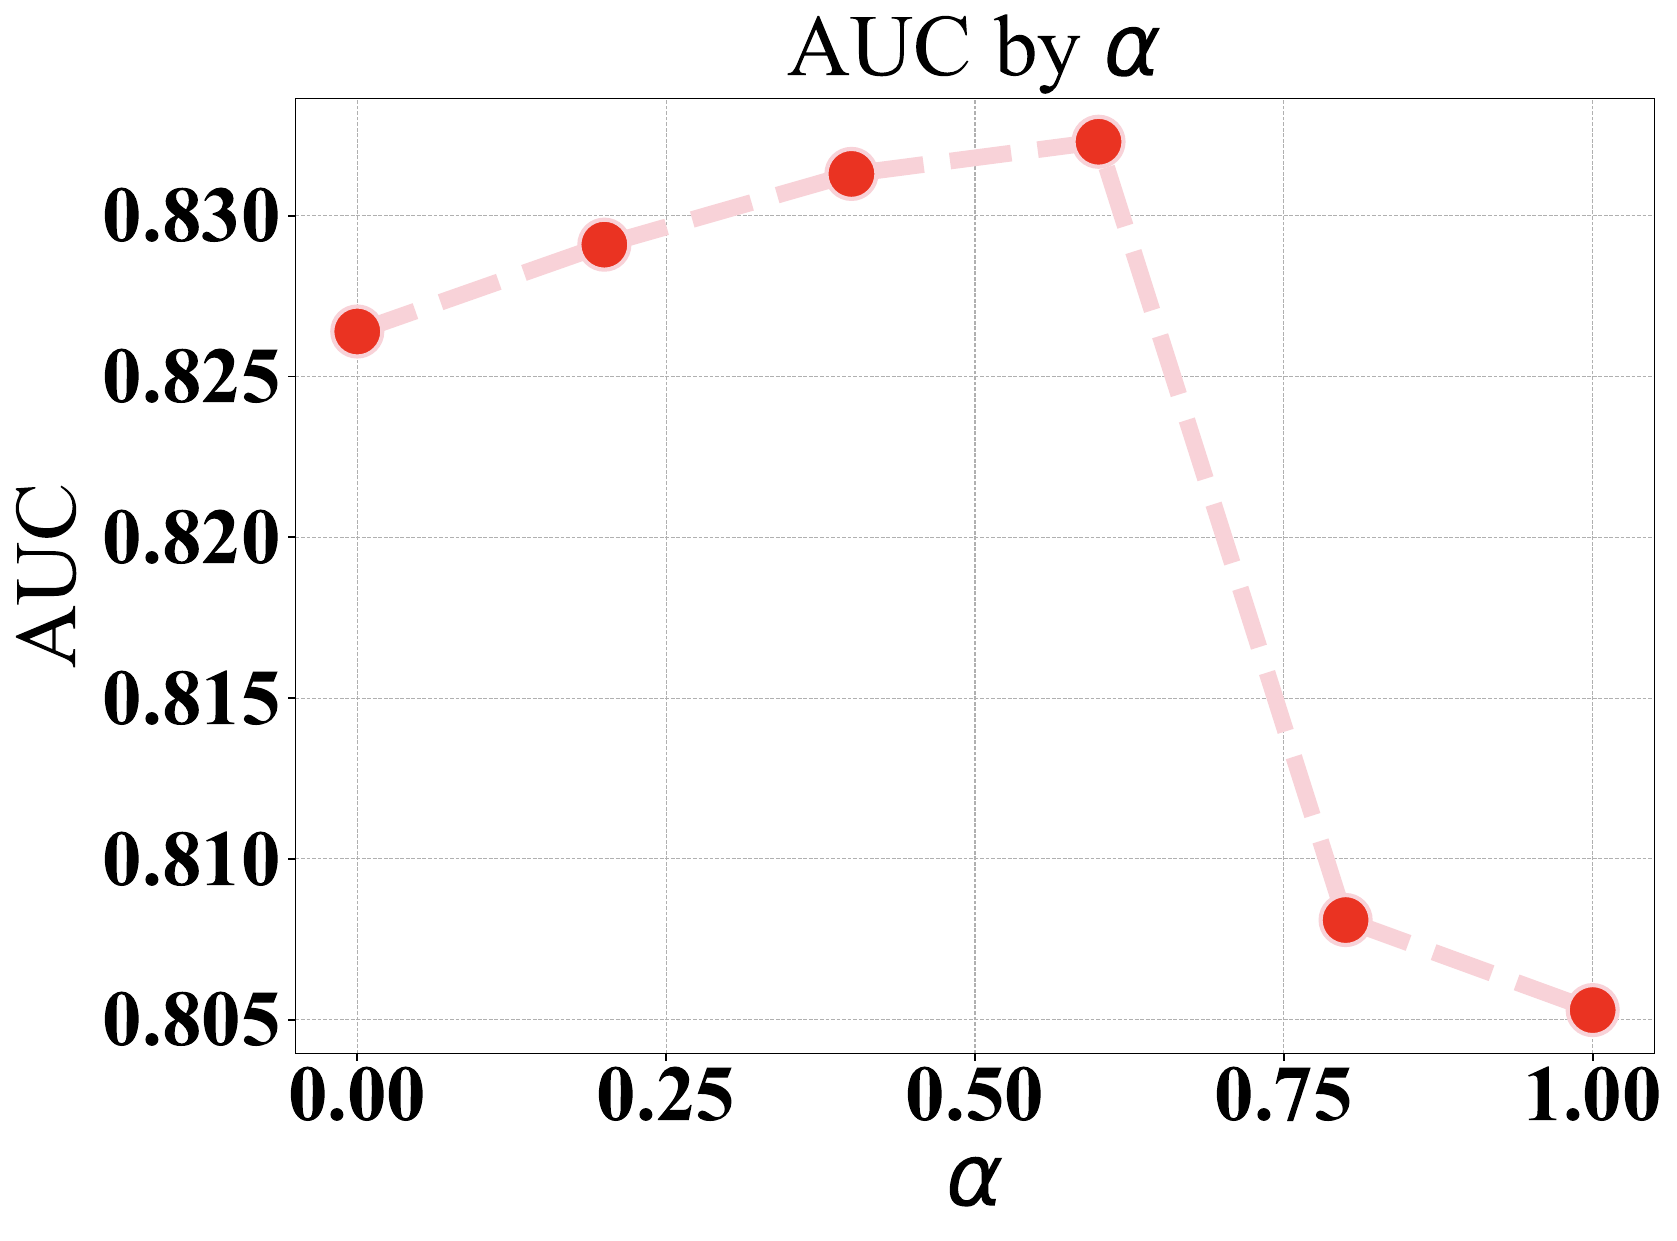}
    \caption[Comparison of AUC scores across varying \(\alpha\) values on Taobao]{Comparison of AUC scores across varying \(\alpha\) values on Taobao. At \(\alpha = 0\), only Retrieval Imitation loss is utilized, whereas at \(\alpha = 1\), only the Contrastive Regularization loss is applied.} % The short caption without math mode can be used in the list of figures
    \label{fig:alpha_values}
\end{figure}

% \begin{figure}[H]
%     \centering
%     \includegraphics[width=0.7\linewidth, height=\textheight, keepaspectratio]{figures/03Experiments/Hyper/Taobao_AUC_by_layers.pdf}
%     \caption{Comparison of AUC scores across varying numbers of Knowledge Encoder MLP layers on Taobao.}
%     \label{fig:mlp_layers}
% \end{figure}
